# Supplementary material for: Adiabatic Quantum Zeno Dynamics of Bosonic Atom Pairs with Large Inelastic Losses
Source: arXiv:2207.02080 ancillary file (2022-07-05)
Supplement: Supplementary file 1 [file SM_ZenoAtomPairs_sub.pdf]

# Supplemental Material for : Adiabatic Quantum Zeno Dynamics of Bosonic Atom Pairs with Large Inelastic Losses

Manel Bosch Aguilera[1], Alexis Ghermaoui[1], Rémy Vatré[1], Raphaël Bouganne[1], Jérôme Beugnon[1], Fabrice Gerbier[1]
[1]*Laboratoire Kastler Brossel, Collège de France, CNRS, ENS-PSL University, Sorbonne Université, 11 Place Marcelin Berthelot, 75005 Paris, France*
(Dated: July 5, 2022)

## I. DETAILED DERIVATION OF THE NON-HERMITIAN HAMITONIAN FROM A LINDBLAD MASTER EQUATION

The dynamics of atom pairs as a competition between coherent laser driving, elastic on-site interactions and two-body losses is described by a master equation

$$\frac{d\hat{\rho}}{dt} = \frac{1}{\mathrm{i}\hbar}\left[\hat{H}_{\mathrm{eff}}, \hat{\rho}\right] + \sum_{\alpha} \Gamma_\alpha \, \hat{L}_\alpha \, \hat{\rho} \, \hat{L}_\alpha^\dagger.$$

Here $\hat{\rho}$ is the density matrix, $\hat{H}_{\mathrm{eff}}$ is the effective Hamiltonian. The jump operators $\hat{L}_i = \hat{a}_{e,i}^2/\sqrt{2}$ describe two-body inelastic losses at site $i$ as quantum jumps from a doubly-occupied Fock state to the vacuum at a rate $\Gamma_{ee} \equiv \Gamma_i$. Here, $\hat{a}_{e,i}$ (respectively, $\hat{a}_{g,i}$) is the annihilation operator for an atom at lattice site $i$ in internal state $e$ (resp., $g$), and $\hat{n}_{e,i} = \hat{a}_{e,i}^\dagger \hat{a}_{e,i}$ (resp., $\hat{n}_{g,i}$) the corresponding number operator. Neglecting inter-sites tunneling, the effective Hamiltonian decomposes as a sum of on-site Hamiltonians $\hat{H} = \sum_i \hat{h}_{\mathrm{eff}}^{(i)}$, with

$$\hat{h}_{\mathrm{eff}}^{(i)} = \hat{h}_{\mathrm{sp}}^{(i)} + \hat{h}_{\mathrm{int}}^{(i)} - \mathrm{i}\frac{\hbar\Gamma_{ee}}{2}\hat{L}_i^\dagger \hat{L}_i. \tag{1}$$

Here,

$$\hat{h}_{\mathrm{sp}}^{(i)} = -\hbar\delta\hat{n}_{e,i} + \frac{\hbar\Omega}{2}\left(\hat{a}_{e,i}^\dagger \hat{a}_{g,i} + \mathrm{h.c.}\right), \tag{2}$$

is a single-particle Hamiltonian describing the laser driving in the rotating-wave approximation, and

$$\hat{h}_{\mathrm{int}}^{(i)} = \sum_{\alpha=e,g} \frac{U_{\alpha\alpha}}{2}\hat{n}_{\alpha,i}(\hat{n}_{\alpha,i} - 1) + U_{eg}\hat{n}_{g,i}\hat{n}_{e,i} \tag{3}$$

is the interaction Hamiltonian with $U_{\alpha\beta}$ the interaction strength between two atoms in states $\alpha, \beta$ at the same lattice site.

The Hamiltonian is a direct sum over sites and we take the initial state to be a product of Fock states. The global density matrix factorizes, $\hat{\rho} = \prod_{\mathrm{sites}\, i} \hat{\rho}^{(i)}$. To discuss the behavior of the on-site density matrices $\hat{\rho}^{(i)}$, we must separate the cases of doubly- and singly-occupied sites. In the following we omit site indices for simplicity.

For doubly-occupied sites, initially in state $|gg\rangle$, the on-site density matrix reads $\hat{\rho}^{(i)} = \hat{\rho}^{(N=2)} + p_\varnothing |\varnothing\rangle\langle\varnothing|$. Here, $\hat{\rho}^{(N=2)}$ is the projection on the 2−particles sector, spanned by the states $\sqrt{2}|gg\rangle = (\hat{a}_g^\dagger)^2|\varnothing\rangle$, $|eg\rangle = \hat{a}_e^\dagger \hat{a}_g^\dagger|\varnothing\rangle$ and $\sqrt{2}|ee\rangle = (\hat{a}_e^\dagger)^2|\varnothing\rangle$. We denote by $|\varnothing\rangle$ the vacuum state (0−particle sector), and $p_\varnothing = 1 - \mathrm{Tr}[\hat{\rho}^{(N=2)}]$ the probability to find the vacuum state. The evolution of $\hat{\rho}^{(N=2)}$ is determined by the effective Hamiltonian alone, while quantum jumps result in irreversible transfer from the 2−particles sector to the vacuum. Using the representation $\hat{\rho}^{(N=2)} = |\Psi^{(N=2)}\rangle\langle\Psi^{(N=2)}|$, the evolution of the (unnormalized) state vector $|\Psi^{(N=2)}\rangle$ is determined by a non-Hermitian Schroedinger equation,

$$\mathrm{i}\hbar\frac{d}{dt}|\Psi^{(N=2)}\rangle = \hat{h}_{\mathrm{eff}}|\Psi^{(N=2)}\rangle. \tag{4}$$

This corresponds to the non-Hermitian dynamics of atoms pairs described in the main text.

For singly-occupied sites, the density matrix only explores the 1−particle sector, $\hat{\rho}^{(N=1)} = |\Psi^{(N=1)}\rangle\langle\Psi^{(N=1)}|$. The state vector $|\Psi^{(N=1)}\rangle$ is a normalized quantum state evolving through the regular Schroedinger equation

$$\mathrm{i}\hbar\frac{d}{dt}|\Psi^{(N=1)}\rangle = \hat{h}_{\mathrm{sp}}|\Psi^{(N=1)}\rangle \tag{5}$$

corresponding to the single-particle Hamiltonian $\hat{h}_{\mathrm{sp}}$. The associated physics corresponds to the standard adiabatic evolution of a two-level system initially in $|g\rangle$, which appears as a parasitic signal on top of the atom pairs signal of interest.

## II. NON-HERMITIAN QUANTUM MECHANICS

In this Section, we give for self-completeness a minimal summary of the main notions in a non-Hermitian generalization of quantum mechanics. A much broader account can be found in Refs. [1, 2]. We consider the spectrum of a finite-dimensional non-Hermitian Hamiltonian $\hat{H}$. We *assume* that $\hat{H}$ is diagonalizable, *i.e.* admits complete sets of right and left eigenvectors $|u_i\rangle$ and $\langle v_j|$ obeying respectively

$$\hat{H}|u_i\rangle = \lambda_i|u_i\rangle, \qquad \hat{H}^\dagger|v_i\rangle = \kappa_i^*|v_i\rangle. \tag{6}$$

In the following, we assume that this spectrum is non-degenerate. Noting that $\langle v_i|\hat{H}|u_j\rangle = \kappa_i\langle v_i|u_j\rangle = \lambda_j\langle v_i|u_j\rangle$, we then deduce *(i)*, that $\langle v_i|u_j\rangle = 0$ for $i \neq j$, and *(ii)*, that the left and right eigenvectors are associated to the *same* eigenvalue $\kappa_i = \lambda_i$. In addition, one can show that the right eigenvectors $|u_i\rangle$ (or the left ones $|v_i\rangle$) form a minimal and complete set of linearly independent vectors [1]. The set $\{|u_i\rangle, |v_i\rangle\}_{i=1,\cdots,N}$ is called a *bi-orthogonal basis*.

Any transformation of the form

$$|u_i\rangle \to a_i(\zeta)|u_i\rangle, \qquad \langle v_i| \to b_i(\zeta)\langle v_i|. \tag{7}$$

leaves the orthogonality and closure relations unchanged. Such transformations can be seen as the generalization of

gauge transformations of Hermitians systems. It is convenient to choose the two independent normalization factors such that $\langle v_i|u_i\rangle = \langle u_i|u_j\rangle = 1$.

The non-Hermitian generalization of a projector is $\hat{P}_i = |u_i\rangle\langle v_i|$ with the chosen normalization $\langle v_i|u_i\rangle = 1$. These projectors enable to generalize the closure relation, $\mathbf{1} = \sum_i \hat{P}_i$, and to express the Hamiltonian in diagonal form, $\hat{H} = \sum_i \lambda_i \hat{P}_i$. The trace of an operator can be expressed in a regular orthonormal basis $\{|\alpha\rangle\}$, and then converted to a bi-orthogonal basis by inserting two closure relations. This yields

$$\mathrm{Tr}\left(\hat{O}\right) = \sum_i \langle v_i|\hat{O}|u_i\rangle. \tag{8}$$

In order to clarify the rule to use to evaluate expectation values of observables, we take a step back and remark that by definition, the non-Hermitian Hamiltonian rules the evolution of the density matrix according to

$$\mathrm{i}\hbar\frac{d\hat{\rho}_1}{dt} = \hat{H}\hat{\rho}_1 - \hat{\rho}_1\hat{H}^\dagger + \cdots, \tag{9}$$

where the elllipsis corresponds to the jump terms assumed negligible or unimportant. Note that $\hat{\rho}_1$ in Eq. (9) is *not* normalized to 1. The "density matrix" $\hat{\rho}_1$ can be represented as

$$\hat{\rho}_1 = |\Psi\rangle\langle\Psi|, \tag{10}$$

with a wavevector $|\Psi\rangle$ obeying the non-Hermitian Schroedinger equation $\mathrm{i}\hbar\, d|\Psi\rangle/dt = \hat{H}|\Psi\rangle$. The expectation value of an observable $\hat{O}$ is then

$$\langle\hat{O}\rangle = \mathrm{Tr}\left(\hat{\rho}_1\hat{O}\right) = \langle\Psi|\hat{O}|\Psi\rangle. \tag{11}$$

The time-evolved quantum state after an evolution time $T$ is

$$|\psi(T)\rangle = \sum_i c_i e^{-\frac{\mathrm{i}\lambda_i T}{\hbar}}|u_i\rangle, \tag{12}$$

where we considered the case of a time-independent Hamiltonian $\hat{H}$. Note that the normalization of $|\Psi\rangle$ is *not* conserved in general since the imaginary part of $\lambda_i$ is not necessarily zero: one particular eigenmode $i$ can thus experience gain or losses depending on the sign of $\mathrm{Im}(\lambda_i)$.

In our particular case, the non-Hermitian Hamiltonian is symmetric, such that $\hat{H}^\dagger = \hat{H}^*$ and $|v_j\rangle = |u_j^*\rangle$. As a result, we only discuss explicitely right eigenvectors in the main text.

## III. DETAILS ON POPULATION MEASUREMENTS

After the preparation ramp, we measure the populations using absorption imaging after a time of flight of 12 ms. We use one of three different protocols accessing different observables: *(i)* imaging using light resonant on the $^1\mathrm{S}_0$-$^1\mathrm{P}_1$ transition. This gives access to the total number of atoms in the ground state $N_g$; *(ii)* imaging on the same transition but after a repumper pulse resonant with the $^3\mathrm{P}_0$- $^3\mathrm{D}_1$ transition. The repumper pulse transfers the atoms from $e$ to $g$ with a measured efficiency $\eta_{\mathrm{rp}} \approx 0.8$. This gives (approximately due to the imperfect repumping) access to the total atom number, $N_g + \eta_{\mathrm{rep}}N_e$; *(iii)* imaging after a "cleaning pulse" resonant on the $^1\mathrm{S}_0$- $^1\mathrm{P}_1$ transition followed by a repumper pulse. The cleaning pulse imparts a momentum kick to $g$ atoms (strong enough to expel them from the trap) while leaving atoms in $e$ essentially unaffected. This protocol thus measures the atom number in the excited state times the repumping efficiency, $\eta_{\mathrm{rp}}N_e$.

## IV. SMALL DEVIATIONS FROM ADIABATICITY IN THE LANDAU-ZENER RAMPS

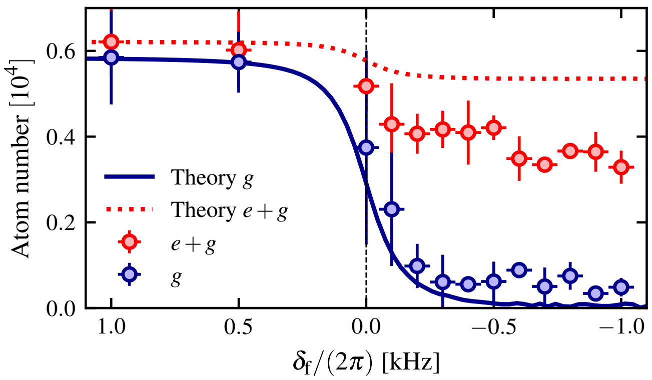


FIG. S1. Landau-Zener ramp for a unit-filled Mott insulator with a single $\bar{n} = 1$ domain. The graph shows the total atom number and $g$ population following the one-atom dressed state connecting to $|g\rangle$ (respectively, $|e\rangle$) for large and positive (resp. negative) detunings. The experiment is performed using a descending frequency ramp at constant speed $\dot{\delta}$, as in the main article. Note that the frequency axis is reversed, so that the ramp time increases from left to right.

### A. Imperfect Landau-Zener passage at large negative detunings

In Fig. 4a in the main text, small deviations from quasi-adiabaticity for negative detunings $\delta_\mathrm{f}$ can be observed. For descending frequency ramps as in Fig. 4a, negative detunings correspond to ramps that have crossed the resonance, but also to longer total evolution times since the ramps are performed at constant speed. For detunings $\delta_\mathrm{f}/(2\pi) \geq 0.25$ kHz, where the deviations are the strongest, the majority of doubly-occupied sites have decayed. We show an additional curve in Fig. S1. The main difference from the experiments reported in the main text is the initial atomic distribution. Here we use an atomic sample with reduced atom number, such that there is essentially only a single Mott region with unit filling. Other parameters are as reported in the main text. Fig. S1 shows the population in $g$ and the total atom number for each final detuning $\delta_f$. Similar deviations from adiabatic behavior can be noted for negative detunings in Fig. S1 as in Fig. 4a: in both cases, a small fraction of the atoms remains in $g$ whereas a

completely adiabatic ramp should transfer all atoms from $g$ to $e$. The adiabatic criterion $\dot{\delta} \ll \Omega^2$ is reasonably well fulfilled, with $\dot{\delta} \approx (2\pi \times 40)^2\,\mathrm{s}^{-2}$ and $\Omega \approx 2\pi \times 150\,\mathrm{s}^{-1}$. The two measurements point to a cause of the negative-$\delta_\mathrm{f}$ deviations that affects singly-occupied sites independently from the non-Hermitian dynamics in the central doubly-filled Mott core.

We believe these deviations originate from experimental noise affecting the laser drive. Experimentally, the dominant noise corresponds to frequency fluctuations of the driving laser $\omega_L(t) + \zeta(t)$, where the mean laser frequency $\omega_L$ eventually depends *deterministically* on time and $\zeta$ is a classical stochastic variable with zero mean. Qualitatively, such fluctuations are expected to make the adiabatic passage for singly-occupied sites imperfect, thus leading to a residual $g$ population for large negative $\delta_\mathrm{f}$. It is difficult to be fully quantitative because we have no means to characterize the laser noise spectrum. Assuming a white spectrum for simplicity, we are able to reproduce the measured negative-$\delta_\mathrm{f}$ deviations by assuming a noise level of $\sqrt{\langle \zeta^2 \rangle} \sim 2\pi \times 10\,\mathrm{Hz}$. This value is realistic for our experimental setup and consistent with Ramsey spectroscopy measurements to be presented elsewhere [3].

### B. Enhancement of noise-driven transitions in the Zeno regime

In Fig. 4a in the main text, one may also notice increased of fluctuations near resonance. In this Section, we consider the frequency noise of the laser drive and show that a non-Hermitian system in the Zeno regime is more sensitive to such fluctuations in comparison to its Hermitian counterpart.

We model frequency fluctuations of the driving laser $\omega_L(t) + \zeta(t)$, where the mean laser frequency $\omega_L$ depends *deterministically* on time and $\zeta$ is a classical stochastic variable, taken to be stationary and with zero mean. The non-Hermitian Hamiltonian becomes $\hat{H}_\mathrm{eff}(t) + (\hbar\zeta(t)/2)\hat{V}$, with a static $\hat{V} \equiv -\hat{S}_z$. To isolate more clearly the noise-induced dynamics, we consider a situation where the system occupies the least dissipative eigenstate $\alpha$ at $t = 0$, and a constant mean laser frequency $\omega_L$ (thus, $\hat{H}_\mathrm{eff}$ is stationary). We write the state vector for $t > 0$ in the eigenbasis of $\hat{H}_\mathrm{eff}$, $|\Psi\rangle = \sum_i c_i(t) e^{-\frac{\mathrm{i}\lambda_i t}{\hbar}} |\lambda_i\rangle$, with $c_i(0) = \delta_{i\alpha}$. The non-Hermitian Schroedinger equation leads to

$$\dot{c}_{i\neq\alpha} = -\frac{\mathrm{i}}{2} \sum_{i\neq\alpha} V_{\alpha i} e^{\mathrm{i}\Omega_{i\alpha}(t)} \zeta(t) c_i(t), \tag{13}$$

with $V_{\alpha i} = \langle \lambda_\alpha^* | \hat{V} | \lambda_i \rangle$ and $\Omega_{i\alpha}(t) = (\lambda_i - \lambda_\alpha)t/\hbar \equiv \omega_{i\alpha} - \mathrm{i}\kappa_{i\alpha}$ a generalized Bohr frequency (note that $\kappa_{i\alpha} \geq 0$ since $\alpha$ is the least dissipative eigenstate).

We now evaluate perturbatively the noise-averaged rate of transitions out of state $\alpha$. Standard algebra leads to $\dot{\bar{c}}_\alpha = -\frac{\gamma_\alpha}{2} - \mathrm{i}\Delta_\alpha$, where the bar denotes noise averaging and where half the dephasing rate $\gamma_\alpha/2$ and the level shift $\Delta_\alpha$ are the real and imaginary parts of

$$I_\alpha = \frac{1}{4} \sum_{i\neq\alpha} |V_{\alpha i}|^2 \int_0^{+\infty} C_\zeta(\tau) e^{(\mathrm{i}\omega_{\alpha i} - \kappa_{i\alpha})\tau} d\tau. \tag{14}$$

Here $C_\zeta(\tau) = \overline{\zeta(t)\zeta(t-\tau)}$ stands for the noise correlation function. In the non-dissipative limit where $\kappa_{i\alpha} \to 0$, the transition rates are determined by the spectral density $S_\zeta(\omega)$, equal to the Fourier transform of the time correlation function by the Wiener-Khintchin theorem, *i.e.* $C_\zeta(\tau) = \int_{-\infty}^{+\infty} d\omega e^{-\mathrm{i}\omega\tau} S_\zeta(\omega)$. More generally, the transition rates are determined by the convolution product

$$\gamma_\alpha = 2 \sum_{i\neq\alpha} |V_{\alpha i}|^2 \int_{-\infty}^{+\infty} \frac{\kappa_{i\alpha} S_\zeta(\omega)}{(\omega - \omega_{\alpha i})^2 + \kappa_{i\alpha}^2} d\omega. \tag{15}$$

When the noise correlation time $\tau_c$ is small compared to the inverse decay rates $\kappa_{i\alpha}^{-1}$, the Lorentzian function in Eq. (15) behave as ($\pi$ times) a delta function when convolved with $S_\zeta$. This leads to the "golden rule" formula

$$\gamma_\alpha \approx 2\pi \sum_{i\neq\alpha} |V_{\alpha i}|^2 S_\zeta(\omega_{\alpha i}) \tag{16}$$

The transition rate is determined by the noise spectral density $S_\zeta$ evaluated at the *real* Bohr frequencies of the considered system, *i.e.* the real parts of the generalized energies $\lambda_i$. In the regime of weak dissipation, the real Bohr frequencies display avoided crossings and are on the order of the coupling strength $\Omega$. On the other hand, in the Zeno regime of strong dissipation, unavoided crossings arise instead and the real Bohr frequencies vanish. As a result, the ratio between the noise-induced decay rates in the two regimes is roughly given by

$$\frac{\gamma_\alpha^\mathrm{Zeno}}{\gamma_\alpha^\mathrm{weak}} \sim \frac{S_\zeta(0)}{S_\zeta(\Omega)} \gg 1, \tag{17}$$

where we assumed that $S_\zeta(\omega)$ increases with decreasing frequency (thereby neglecting pathological situations). We conclude that a non-Hermitian system in the Zeno regime will generally be more sensitive to noise than its weakly dissipative counterpart, with maximum sensitivity near the resonances. This explains qualitatively the large increase of fluctuations when crossing the resonance.


[1] D. C. Brody, Journal of Physics A: Mathematical and Theoretical **47**, 035305 (2013).

[2] Y. Ashida, Z. Gong, and M. Ueda, Advances in Physics **69**, 249 (2020), https://doi.org/10.1080/00018732.2021.1876991.

[3] A. Ghermaoui, R. Vatré, M. Bosch Aguilera, R. Bouganne, I. Fritsche, J. Beugnon, and F. Gerbier, in preparation (2022).
